# Supplementary material for: Rolling, sliding and trapping of driven particles in square obstacle lattices
Source: arXiv:2505.21702 ancillary file (2025-05-27)
Supplement: Supplementary file 1 [file Supplementary-Material.pdf]

## Supplemental Material

# Rolling, sliding and trapping of driven particles in square obstacle lattices

Galor Geva, Arin Escobar Ortiz, Paula Magrinya, Pablo

Llombart, Laura R. Arriaga,<sup>\*</sup> and Juan L. Aragonés<sup>†</sup>

*Department of Theoretical Condensed Matter Physics,*

*Universidad Autónoma de Madrid, 28049, Madrid, Spain*

*Condensed Matter Physics Center (IFIMAC),*

*Universidad Autónoma de Madrid, 28049, Madrid, Spain and*

*Instituto Nicolás Cabrera, Universidad Autónoma de Madrid, 28049, Madrid, Spain*

Alfredo Alexander-Katz

*Department of Materials Science and Engineering,*

*Massachusetts Institute of Technology, Cambridge, MA, 02139, USA*

(Dated: May 27, 2025)

## I. PDMS pattern preparation

The PDMS structure is prepared by cast molding on a master silicon wafer. The master was created using photolithography and was ordered from ELVESIS. Each cylinder has a radius of  $5\mu m$  and a height of  $11.5 \pm 0.5 \mu m$ . A PDMS substrate was then created using a Sylgard 184 silicone elastomer kit (DOW).

### A. Curing

The elastomeric pre-polymer and the crosslinker were mixed at a ratio of 10:1, then poured over the master wafer containing the relief pattern and inserted to an oven at room temperature. It is important to have a thick enough PDMS layer to prevent it from bending while handling it, which might damage the obstacles. On the other hand, the substrate must not be too thick for the working distance of the objective. a thickness of  $\approx 4mm$  proved to be robust enough. The curing stages are as follows: The oven is heated gradually for one hour, until reaching a final temperature of  $65^\circ C$ . Then, the temperature is kept at  $65^\circ C$  for 5 hours of curing. The PDMS mold then cools down gradually inside the oven and left overnight at room temperature.

### B. Coating

The PDMS mold is first peeled off the master wafer, and then immersed in isopropanol and sonicated for  $\sim 2$  minutes. The mold is then rinsed with water, dried gently with compressed air. To increase wettability, the mold is irradiated with oxygen plasma for 60 seconds (Femto-SLS, by Diener) and immediately immersed in a 0.1M PEG-6k aqueous solution (81260, by Sigma-Aldrich) for  $\sim 30$  min. Lastly, the mold is rinsed thoroughly with water, dried gently with compressed air, and stored in a cool and dry area.

---

\* laura.rodriquezarriga@uam.es

† juan.aragones@uam.es

## II. Sample preparation

A sample is prepared by placing  $8\mu L$  of an aqueous colloidal suspension on top of the mold containing the pattern, then closing the sample from above with a coverslip in a sandwich configuration and sealing with a UV-cured optical adhesive (NOA 68, by Norland).

## III. 3D reconstruction of the PDMS structure

3D Imaging of the obstacle lattice was carried out using an inverted confocal fluorescence microscope (Nikon Eclipse Ti) with a 4-laser module (C2Si), and a 40x silicon oil immersion objective (CFI Plan Apo Lambda S 40XC Sil,  $NA = 1.25$ ).  $10\mu L$  of  $20\mu M$  Sulphorhorhodamine-B was placed on top of a thin coverglass, and the substrate was placed face down on the droplet. The 3D reconstruction was carried out using ImageJ [1].

## IV. Image acquisition and signal generation

Using a custom MATLAB script, we generated two sinusoidal signals with a phase shift of  $\pi/2$  and converted them from digital to analog using a DAQ device (Measurement Computing USB-1208HS). The signals were then amplified using 500 W amplifiers (LD Systems). The voltage sent to the coils was monitored with an oscilloscope (Tektronix TDS 2014B). The magnetic field in the Helmholtz configuration was  $\sim 10$  mT for rotation frequencies up to 20 Hz and  $\sim 15$  mT for frequencies up to 40 Hz. To induce rolling along the y-axis, we applied a magnetic field rotating about the x-axis (in the xz-plane) by sending the sinusoidal signals to two Helmholtz coil pairs aligned with the x- and z-axes. Images were acquired at 40 fps (BFLY-PGE-23S6M-C, by FLIR), using a Nikon ECLIPSE Ts2R inverted microscope equipped with a  $40\times$  air objective (Nikon S Plan Fluor ELWD ADM 40XC,  $NA = 0.6$ ) with a tunable working distance.

## V. Free rolling parameter measurements

We examine the free rolling parameter  $\xi_0$ , defined as the rolling parameter of the particles on a PDMS substrate in the absence of obstacles, across the range of particle sizes and rotation frequencies used in our experiments. We find that  $\xi_0$  is independent of the rotation

frequency, for the entire range of rotation frequencies and particle sizes examined, as shown in Fig S1.

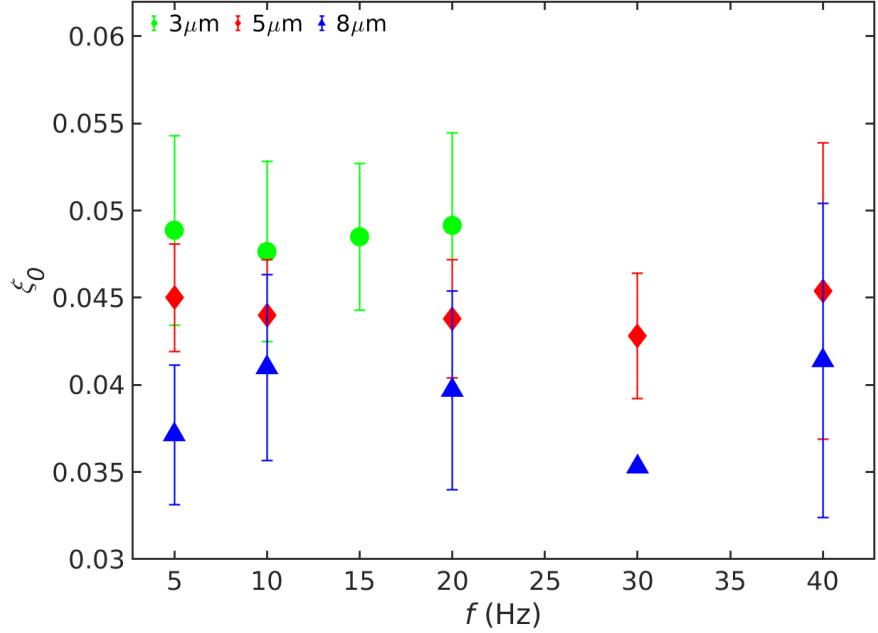

FIG. S1: The free rolling parameter  $\xi_0$  as a function of rotation frequency, for all the particle sizes used. Particle densities are  $1.6 - 1.8 \text{ gr/ml}$ ,  $1.1 - 1.2 \text{ gr/ml}$ , and  $\sim 1.4 \text{ gr/ml}$ , for the 3, 5, and 8 microns respectively.

## VI. Sliding motion analysis for different frequencies and lattice spacings

We examined the sliding velocity as a function of the frequency of rotation and found that it increases linearly with frequency, as shown in Fig S2. In addition, to complement Fig. 4 of the main text, we analyzed the roto-translational coupling parameter for all rotational frequencies and all lattice spacing-to-particle size ratios. In all cases, we observe that sliding is fastest at the center of the unit cell, as shown in Fig S3 consistent with the results presented in the main text.

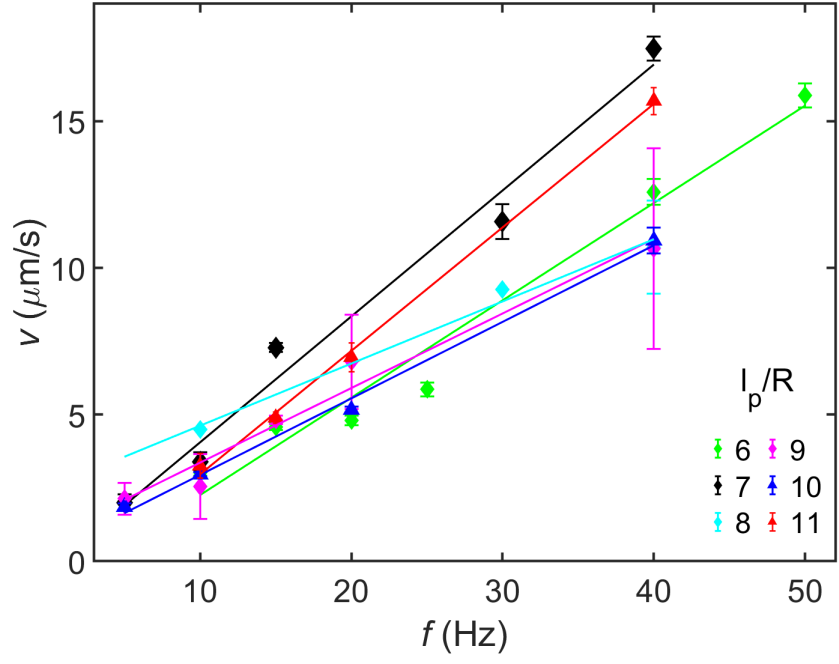

FIG. S2: Sliding velocity vs rotating frequency for all conditions where sliding was observed, for particle sizes of  $5\mu\text{m}$  (diamond) and  $8\mu\text{m}$  (triangle). Linear fits shows strong agreement with the data, with  $R^2 = 0.97, 0.98, 0.99, 0.97, 1, 1$ , respectively.

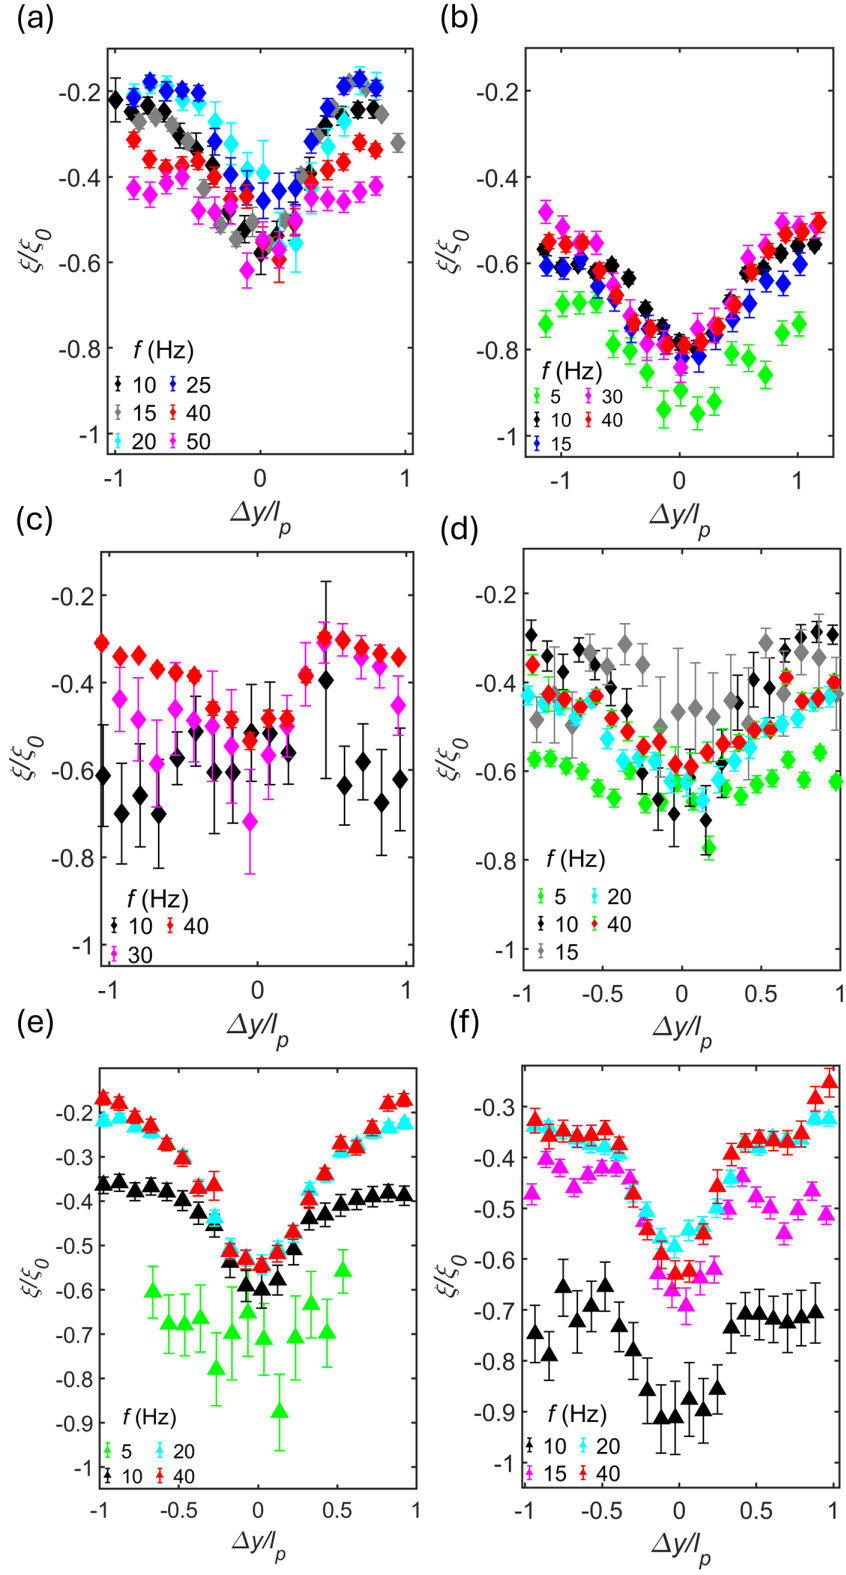

FIG. S3:  $\xi/\xi_0$  vs position inside unit cell, for  $5\ \mu\text{m}$  ( $l_p = 2.4, 2.8, 3.2, 3.6$ ) and  $8\ \mu\text{m}$   $l_p = 2.5, 2.75$  particles, respectively.

## VII. Particle height analysis

The particles were tracked using a standard tracking algorithm that, after applying a band-pass filter to the image, estimates the particle center as the brightest pixel. Then, by fitting to a point-spread function, we find the position of the particle with a sub-pixel accuracy. The intensity of the brightest pixel, as well as the width of the fitted profile, changes as the particle moves along the z-axis, effectively moving in and out of focus. We utilized this to follow minute changes in the particle's position as it moves within the lattice. To calibrate this method, we manually adjusted the focal plane by gently turning the microscope's fine focus knob. First, a thick coverglass (1.2 mm) was used to relate the knob turns to changes in height. A change in a single angular increment (a single tick mark) in the fine microscope knob corresponds to a height change of  $\sim 1.5 \mu m$ . Next, we prepare a PDMS sample, focusing on a single  $5 \mu m$  particle suspended near the substrate. We then manually advanced the knob, a single angular increment at a time, acquired 1000 images for each angle, and extracted the particle's fit width and peak intensity for each batch of images (see Fig S4), thus calibrating variations in particle height to changes in intensity and fit width. To examine the vertical displacement of the particle, we adjust the microscope objective height so that the particle appears slightly out of focus, thus allowing clearer differentiation between upward and downward motion. We then examine the fit width and peak intensity of a particle moving inside the lattice. For example, in the case of oscillatory motion, where the particle alternates between sliding and rolling, we observe that the velocity varies with fit width and peak intensity. Furthermore, we are able to identify the cutoff in which the particle's motion flips direction, as shown in Fig S5.

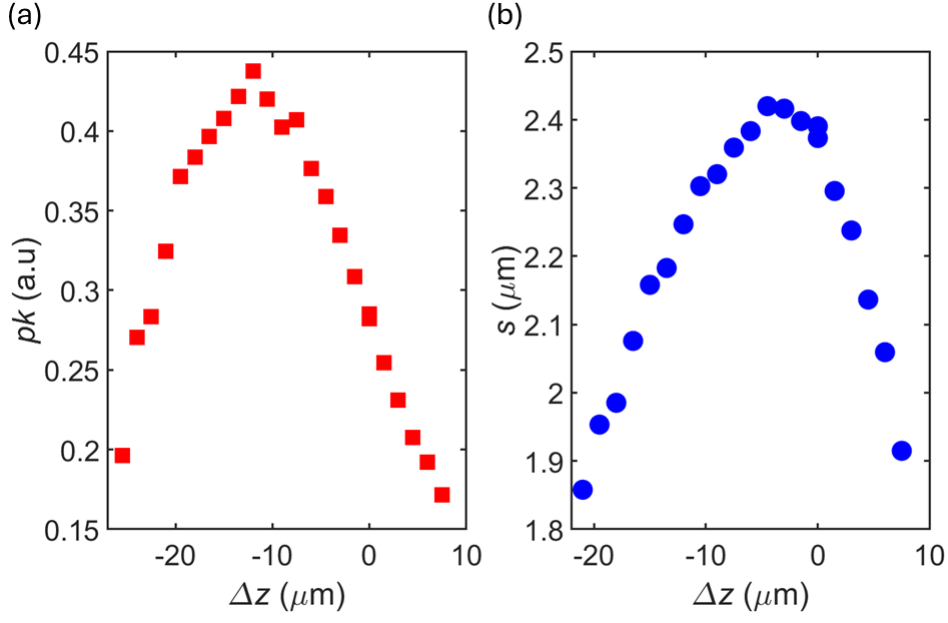

FIG. S4: Peak intensity (a) and fit width (b) vs particle height, for a  $5 \mu\text{m}$  particle.

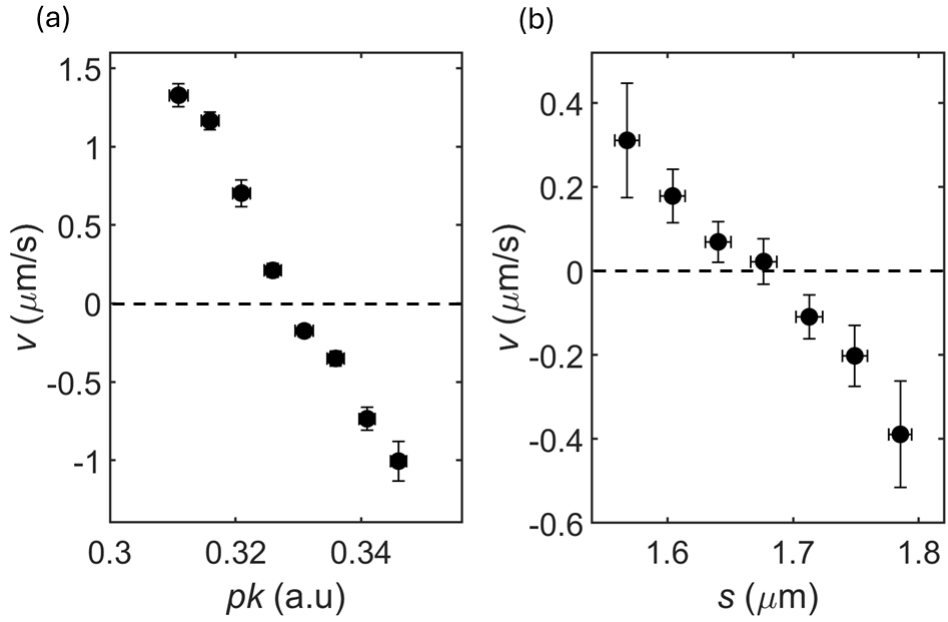

FIG. S5: Analysis of hydrodynamic trapping of  $5 \mu\text{m}$  particles, oscillating within a unit cell ( $l_p/R = 4.4$ ).

Particle velocity vs. the peak intensity (a) and the fit width (b).

### VIII. Simulation methods

To simulate the experimental system, we used a homemade Stokesian Dynamics [2] code written in CUDA/C++. The code uses the Ermak-McKammon algorithm [3] to resolve the particle's motion, with the Rotne-Prager-Yamakawa (RPY) tensor as the mobility matrix. The RPY tensor gives the response in velocity of a sphere  $i$  to a force exerted upon a sphere  $j$ , of equal radii  $a$ ; with relative position  $\vec{r} = \vec{r}_i - \vec{r}_j$ , when immersed in a fluid of viscosity  $\eta$  and in Stokes conditions ( $Re = 0$ ). It takes the following form:

$$\vec{U}_{ij} = \frac{1}{6\pi\eta a} \left\{ \begin{array}{ll} (\frac{3a}{4r} + \frac{a^3}{2r^3})\mathbf{I} + (\frac{3a}{4r} - \frac{3a^3}{2r^3})\hat{r}\hat{r}, & \text{if } i \neq j \text{ and } r \geq 2a, \\ (1 - \frac{9r}{32a})\mathbf{I} + \frac{3r}{32a}\hat{r}\hat{r}, & \text{if } i \neq j \text{ and } r < 2a, \\ \mathbf{I}, & \text{if } i = j \end{array} \right\} \vec{F}_j \quad (1)$$

Thermal noise was calculated using the Krylov subspace approximation [4]. The lubrication correction for close-range hydrodynamic interactions was not included. To resolve the effect of higher-order contributions upon the particle (such as the stresslet or the effect of the velocity gradient) we used the so-called "raspberry model", by which solid bodies are approximated as spherical beads connected by harmonic potentials. It has been shown that the effect of the RPY tensor upon these spherical beads approximates well the effect of higher-order contributions upon the solid body [5]. We chose open boundary conditions to prevent any possible spurious hydrodynamic effects that could arise from the particle interacting with its own images in periodic boundary conditions.

The particle was simulated as a 12-bead assembly, with the beads placed as the vertices of a regular dodecahedron. The obstacles were simulated as 32-bead cylinders, with twice the diameter and 3.2 times the height of the particle. The substrate was simulated as a square bead lattice. The particle beads are connected among themselves with harmonic potentials of equilibrium length equal to the initial bead to bead distance and strength of  $100 k_B T$ . The substrate and obstacle beads are connected among themselves in an identical manner. See figure S6 for a snapshot of a simulation.

To simulate the particle's rotation, a "magnetic dipole"  $\vec{m}$  of the particle was defined as a vector connecting two diametrically opposed beads. In our case, we chose the pair with maximum and minimum  $z$  in the initial configuration, so that the particle's magnetic dipole is initially parallel to the  $z$  axis. A magnetic field vector  $\vec{B}$  was defined as rotating in the

$yz$  plane with fixed amplitude and frequency. The torque the field exerts on the particle is therefore  $\vec{\tau} = \vec{B} \times \vec{m} = B_0(0, \sin(\omega t), \cos(\omega t)) \times \vec{m}$ . This torque is subsequently spread as forces over the 12 beads that compose the particle before carrying out the integration step.

The pressure was calculated using the Oseen point-force approximation, by which the pressure caused in  $\vec{x}$  by a point force  $\vec{F}$  situated at the origin is given by  $P = \frac{\vec{F} \cdot \vec{x}}{4\pi x^3}$ . The approximation for pressure used is singular at short distances, so the pressure on the points closest to the beads is artificially set to zero to avoid high, unrealistic values.

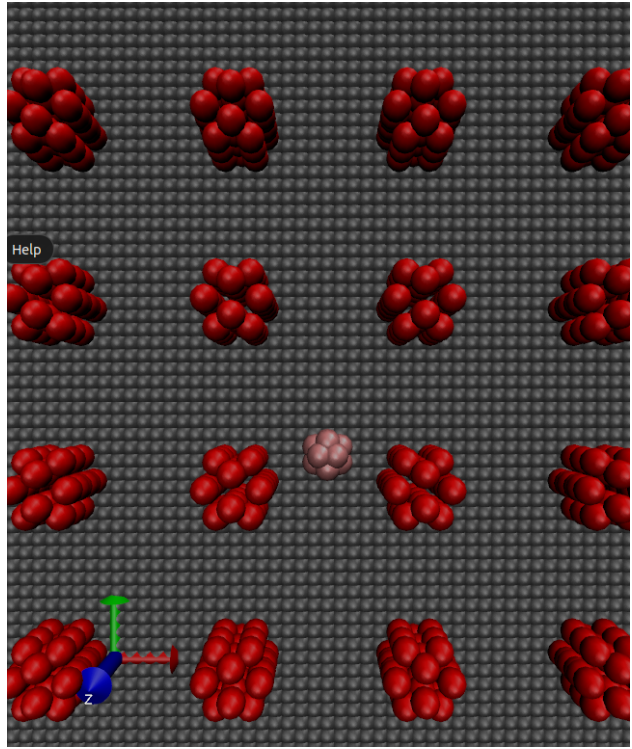

FIG. S6: A snapshot of a visual render of one of the RPY simulations used. Beads composing the obstacles are drawn in red; beads composing the particle are drawn in pink and beads composing the substrate are drawn in gray. The beads composing the substrate and obstacles are linked between them with harmonic potentials. The beads composing the particle are linked likewise. This snapshot was generated with VMD. VMD is developed with NIH support by the Theoretical and Computational Biophysics group at the Beckman Institute, University of Illinois at Urbana-Champaign.

## IX. Dependence of coupling parameter on particle height

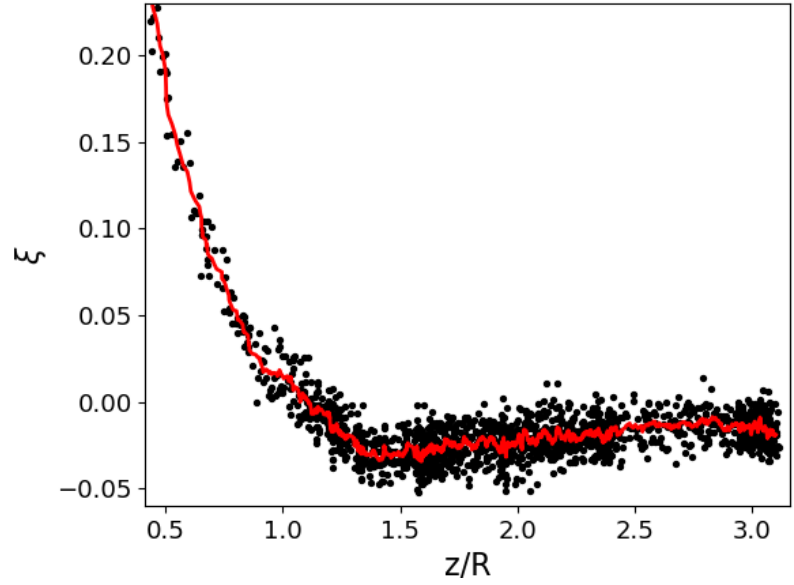

FIG. S7: Instantaneous coupling parameter  $\xi$  versus particle height above the substrate for a continuous RPY simulation where the  $z$  coordinate of the particle was permitted to evolve freely. It can be seen that these results qualitatively agree with those on figure 4c. The higher level of noise in this figure is due to the instantaneous nature of the estimations of  $\xi$ , as opposed to those on figure 4c, where each point is an average over several short simulations. The red line is a running average of 15 data point intervals, included to guide the eye.

## X. Visualization of pressure forces at different positions within the unit cell

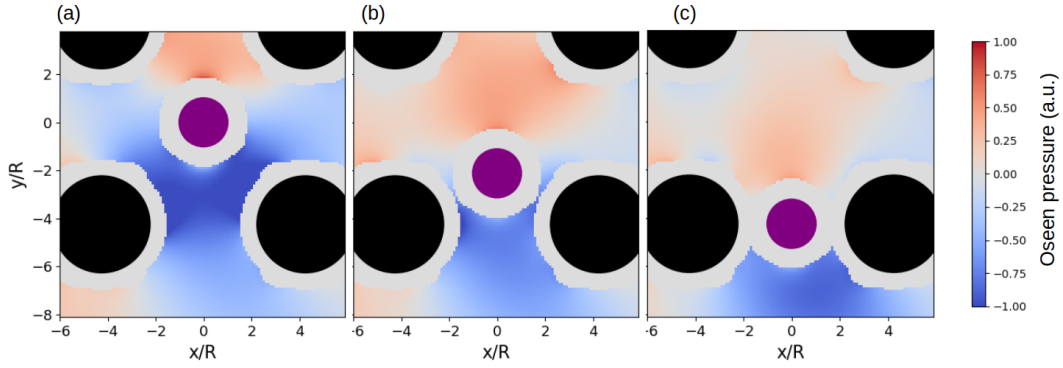

FIG. S8: Approximation of the pressure fields in the XY plane at  $z/R = 1.5$  and  $l_p/R = 9$  when the particle center is situated at (a)  $y = 0$ , (b)  $y = -l_p/2$  and (c)  $y = -(l_p/2 + R_o)$ . The purple circle represents the particle's hydrodynamic radius and the black circles, the hydrodynamic radii of the obstacles. In all three cases the particle is rotating clockwise around the x axis at 10 Hz. In the gray areas around the particle and obstacles, the pressure has been set to zero to avoid high unphysical values (see simulation methods).

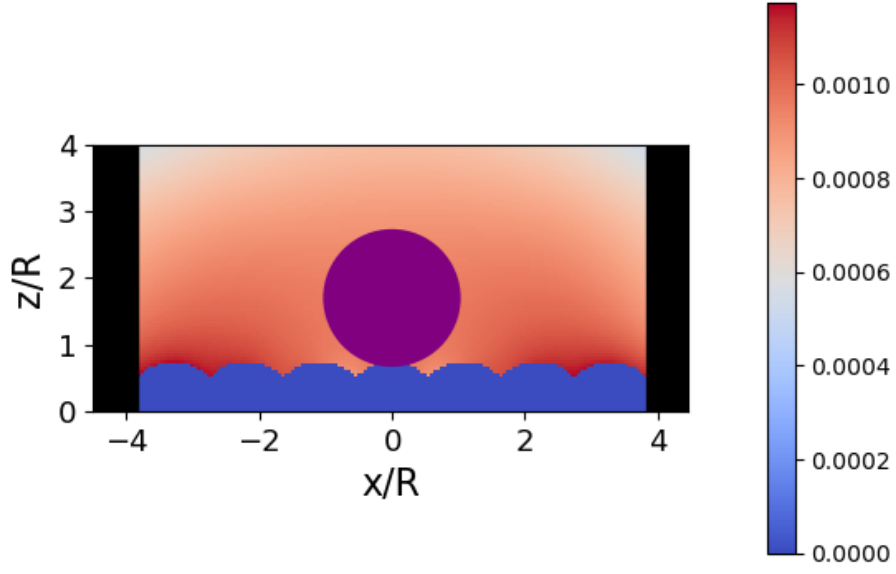

FIG. S9: Approximation of the pressure field in the XZ plane at  $z/R = 2$  and  $l_p/R = 9$  when the particle center is situated at  $y = -(l_p/2 + R_o)$ . The purple circle represents the particle's hydrodynamic radius and the black rectangles, the hydrodynamic radii of the obstacles. The particle is rotating clockwise around the x axis at 10 Hz. The pressure is positive in all the observed area, and decreases for higher  $z$ . This will create a pressure force that pushes the particle farther from the substrate. In the blue areas near the substrate, the pressure has been set to zero to avoid high unphysical values (see simulation methods).

## XI. Supplementary movies

SM1: compares rotating particles both within and outside of the lattice. The "free" particles, i.e., those far from the obstacles, roll to the left, whereas the particle within the lattice slides to the right.

SM2 shows a single sliding particle within the lattice.

SM3 shows a denser magnetic silica particle rolling in the direction of the rotating motion,

due to its proximity to the substrate that results in enhanced shear forces.

SM4 shows a rotating particle oscillating between rolling and sliding motion, effectively being trapped within a single unit cell.

SM5 and SM6 both show simulations of a rotating particle. SM5 shows a simulation of a rotating particle exhibiting rolling motion, and SM6 shows a simulation of a rotating particle exhibiting sliding motion. SM5 and SM6 were rendered using VMD.

- 
- [1] E. E. Diel, J. W. Lichtman, and D. S. Richardson, *Nature Protocols* **15**, 2773 (2020).
  - [2] A. M. Fiore and J. W. Swan, *Journal of Fluid Mechanics* **878**, 544–597 (2019).
  - [3] D. L. Ermak and J. A. McCammon, *The Journal of Chemical Physics* **69**, 1352 (1978).
  - [4] T. Ando, E. Chow, Y. Saad, and J. Skolnick, *The Journal of Chemical Physics* **137**, 064106 (2012), [https://pubs.aip.org/aip/jcp/article-pdf/doi/10.1063/1.4742347/14078473/064106\\_1\\_online.pdf](https://pubs.aip.org/aip/jcp/article-pdf/doi/10.1063/1.4742347/14078473/064106_1_online.pdf).
  - [5] F. B. Usabiaga, B. Kallemov, B. Delmotte, A. Bhalla, B. Griffith, and A. Donev, *Communications in Applied Mathematics and Computational Science* **11**, 217 (2016).
